# Supplementary material for: VEU-Bench: Towards Comprehensive Understanding of Video Editing
Source: arXiv:2504.17828 source file (2025-04-24)
Supplement: Supplementary file 1 [file X_suppl.tex]

\clearpage
\appendix
\setcounter{page}{1}
\maketitlesupplementary

\setcounter{section}{0}
\setcounter{figure}{0}

%%%%%%%%%%%%%%%%%%%%%%%%%%%%%%
\numberwithin{equation}{section}
\numberwithin{figure}{section}

In this supplementary material, we provide a detailed description of the dataset construction process, an in-depth analysis of model performance on VEU-Bench as well as the impact of training data on model performance. Section~\ref{sec: supp_dataset_construction} details the dataset filtering and splitting processes, along with the specific distribution within VEU-Bench. Section~\ref{sec: supp_annotation} presents examples of QA pairs and the details of knowledge base construction. Section~\ref{sec: supp_prompt} provides prompts used for annotation, inference, and evaluation. Section~\ref{sec: supp_train_data} discusses the impact of different proportions of task types on model training. Section~\ref{sec: supp_concept_exp} elaborates on the details of the concept experiments. Section~\ref{sec: supp_analysis} analyzes the model performance on VEU-Bench with a category-wise breakdown. Section~\ref{sec: supp_qualitative samples} showcases visual results and comparisons for each task, while Section~\ref{sec: supp_limitation} discusses the limitations of VEU-Bench and outlines directions for future research.

\section{Dataset Construction Details}
\label{sec: supp_dataset_construction}
\subsection{Curation and Filter}
\noindent
\textbf{Video-wise}: We curated videos from AVE\cite{argaw2022anatomy}, MovieCuts\cite{pardo2022moviecuts}, and AutoTransition\cite{shen2022autotransition}, trimming them into single-shot clips where each clip contains only one editing component. This ensures stable model outputs and focuses recognition on a single type of component. We filtered out videos shorter than 0.5 seconds to ensure sufficient temporal information for recognizing stable editing features. For transitions that occur within a single frame, we trimmed 1-second clips, including 0.5 seconds before and 0.5 seconds after the transition.

\noindent
\textbf{Dimension-wise}: We removed incorrect dimensions, such as \textit{"inter-shot"} in shot type, which cannot be determined through a single clip. For instance, AVE\cite{argaw2022anatomy} only annotates the insert shot itself without including context clips, contradicting the definition of inter-shot. Due to the video understanding limitations of current Vid-LLMs, most of which cannot handle multi-video inputs, we focused on single continuous video clips, which can include either multi-shot or single-shot sequences. We also removed videos with \textit{"other"} labels to ensure a well-defined and clean benchmark.

\noindent
\textbf{Label-wise}: In the AVE\cite{argaw2022anatomy} dataset, there are multi-labeled videos. We transformed some of these into change-detection tasks, verifying labels through Gemini\cite{team2023gemini} and GPT\cite{gpt4o}. Specifically, for change-detection tasks, we sampled the first two frames and the last two frames, requiring both Gemini and GPT to recognize the shot attributes of the changing tasks. Only videos where the labels matched the answers from both GPT and Gemini were retained. For shot-size changes, we only kept evident changes, such as from extreme-wide to medium, and removed subtle changes, such as from extreme-wide to wide. For other tasks, we balanced the label distribution across dimensions in the test set. As shown in Table{}, the original annotations of the AVE and MovieCuts datasets exhibited significant imbalance. We balanced the number of labels to provide more reasonable and effective evaluations, avoiding potential model bias towards single-category answers that could artificially boost accuracy.

\subsection{Split of evaluation data}
For MovieCuts\cite{pardo2022moviecuts} and AutoTransition\cite{shen2022autotransition}, we follow the train and test split from the original datasets and subsample videos from the test set to construction evaluation data of VEU-Bench. For AVE\cite{argaw2022anatomy}, since no split of the datasets is publicly available, we split the AVE datasets with sthe ame portion according to the original paper\cite{argaw2022anatomy} and will make a split of datasets publicly available.

\subsection{Detailed category distribution}
\begin{figure*}[htbp]
    \centering
    \includegraphics[width=\linewidth]{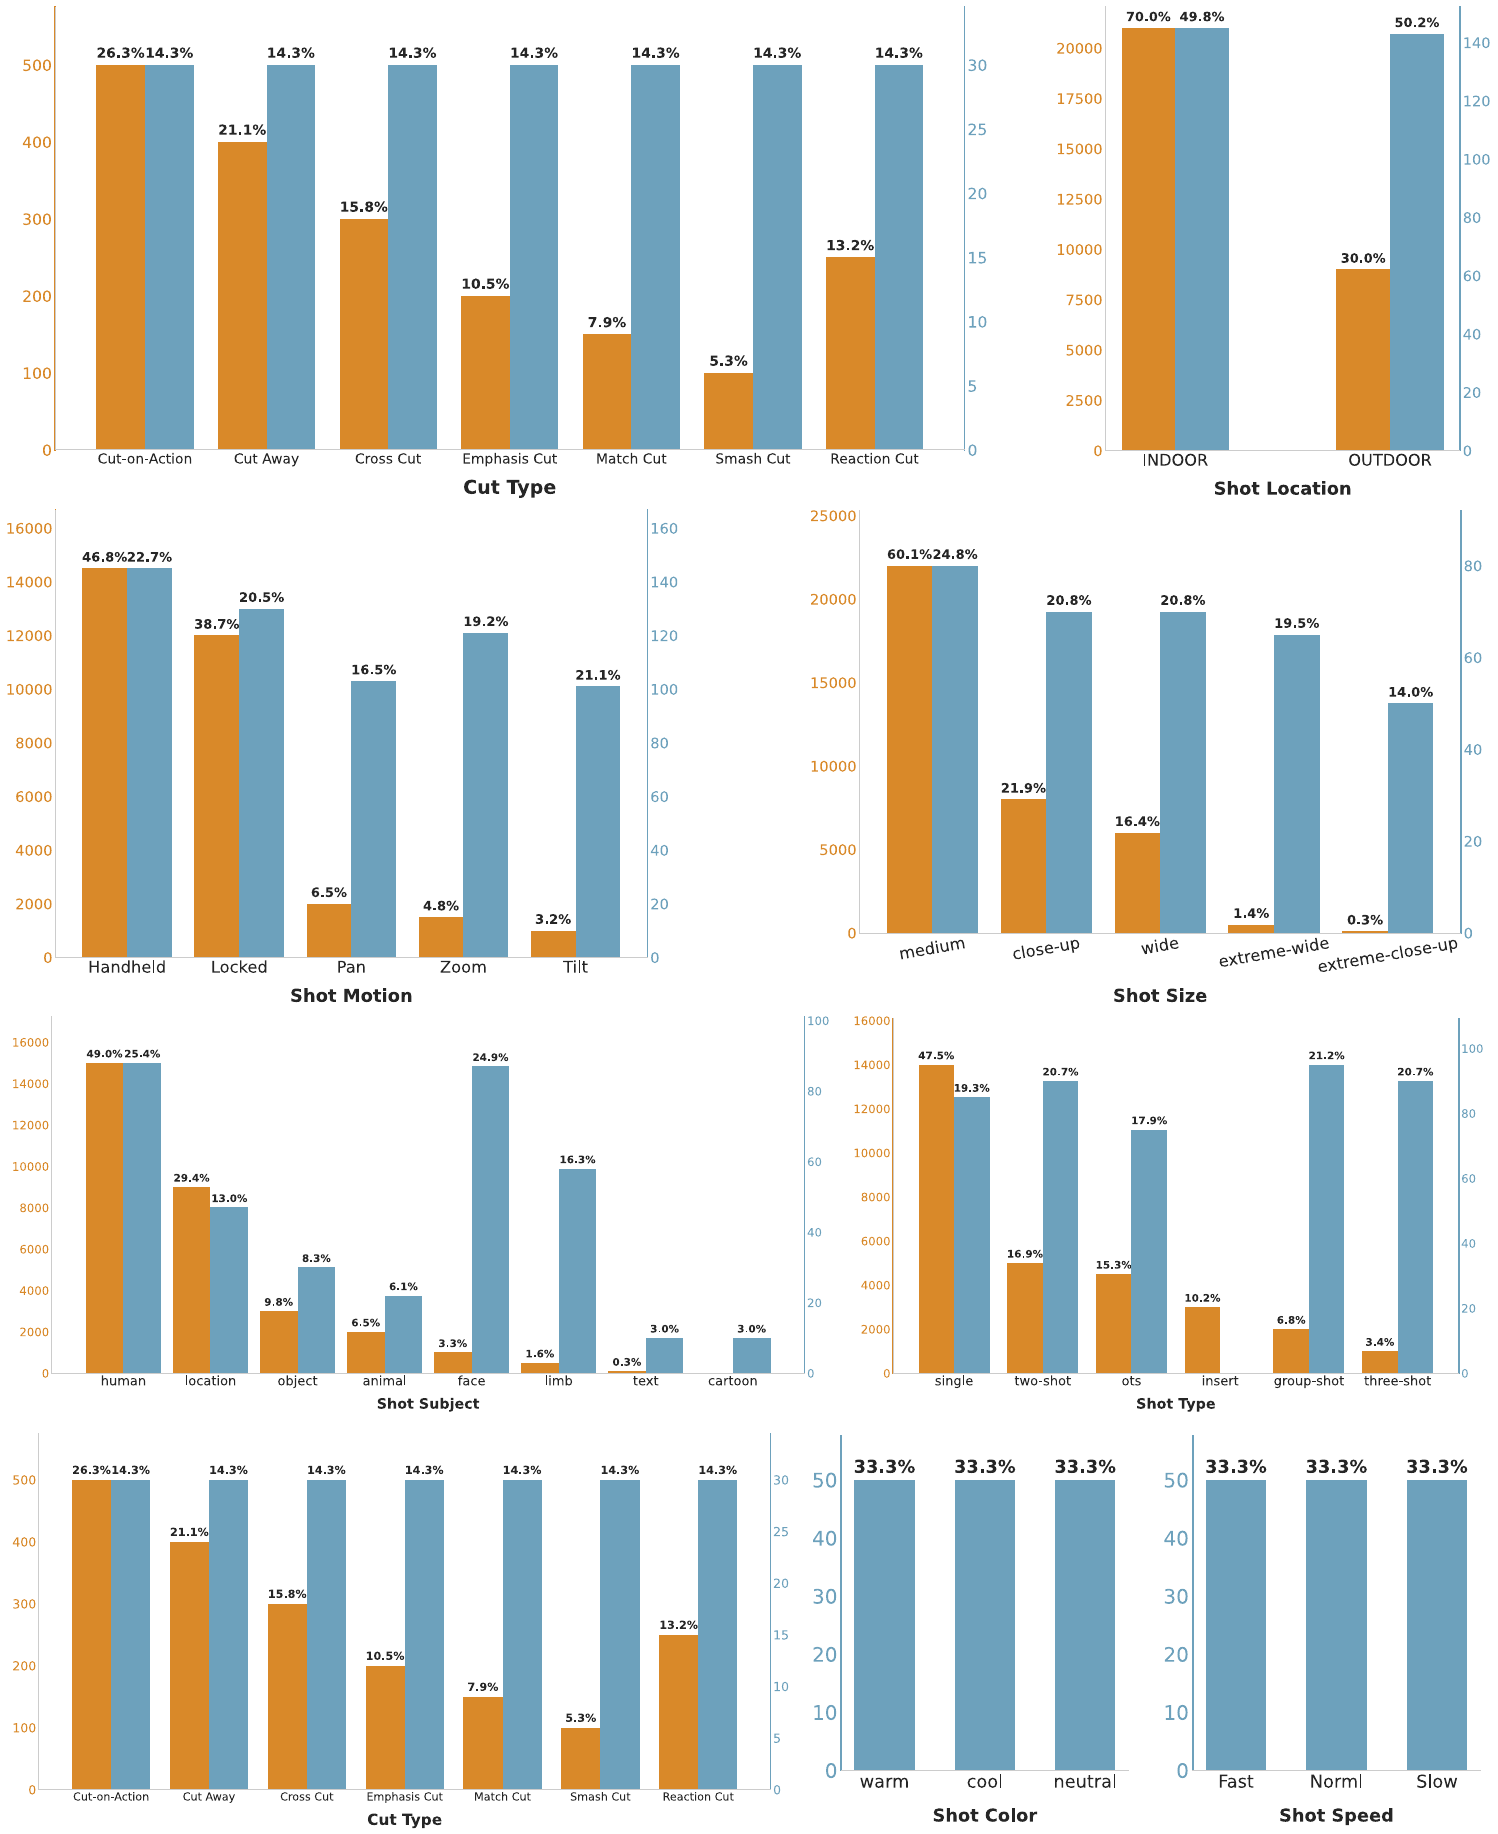}
    \caption{Comparison between the original data distribution (sky blue) and the VEU-Bench evaluation set distribution (deep blue). Zoom in to get the best reading experience.}
    \label{fig:category_distribution}
\end{figure*}

We present the category-wise data distribution of the VEU-Bench evaluation set in Figure~\ref{fig:category_distribution} and compare it with the original distributions from AVE~\cite{argaw2022anatomy}, AutoTransition~\cite{shen2022autotransition}, and MovieCuts~\cite{pardo2022moviecuts}. The imbalance in the original datasets has been significantly reduced, enabling a more stable test setup and trustworthy results, while preventing Vid-LLMs from achieving higher scores by focusing on a single dominant category.

\section{Annotation}
\label{sec: supp_annotation}

\noindent
\textbf{Question List}: We provide the question list of each task in Table~\ref{tab:question_list}. We introduce four questions per task to guarantee diverse input form and stable and general output of the model. 
\begin{table*}[ht]
    \centering
    \small
    \caption{Questions List of VEU-Bench Across 19 tasks. }
    \begin{tabular}{l|p{14cm}}
        \toprule
        \textbf{Dimension} & \textbf{\centering{Questions}} \\ 
        \midrule
        \midrule
        \multicolumn{2}{c}{\textit{Editing Dimension = Shot Color, Shot Speed, Shot Size, Shot Angle, Shot Type, Shot Motion, Shot Location, Shot Subject, Cut Type, Transition}}\\
        \midrule
        \midrule
        Recognition
        & \textbf{(1)} To which \textit{\{Editing Dimension\}} does the given video belong; \textbf{(2)} Determine the \textit{\{Editing Dimension\}} used in the given video; \textbf{(3)} What category of \textit{\{Editing Dimension\}} does the given video represent; \textbf{(4)} Identify the \textit{\{Editing Dimension\}} for the given video. \\
        \midrule
        \midrule
        \multicolumn{2}{c}{\textit{Editing Dimension = Shot Size, Shot Angle, Shot Location}}\\
        \midrule
        \midrule
        Change Reasoning
        & \textbf{(1)} In the given video, identify the \textit{\{Editing Dimension\}} change from one type to another and state the basis for your determination; \textbf{(2)} Based on the given video, specify the \textit{\{Editing Dimension\}} transition from one type to another and provide the criteria for this judgment; \textbf{(3)} In the given video, clarify the \textit{\{Editing Dimension\}} shift from one type to another and explain the clue for this change; \textbf{(4)} For the given video, outline the change in \textit{\{Editing Dimension\}} from one type to another and explain the basis for your decision. \\
        \midrule
        \midrule
        \multicolumn{2}{c}{\textit{Editing Dimension = Shot Motion, Shot Type, Cut Type, Transition}}\\
        \midrule
        \midrule
        Dynamic Reasoning
        & \textbf{(1)} In the given video, clarify the \textit{\{Editing Dimension\}} and explain the grounds for your judgment. \textbf{(2)} For the given video, outline the \textit{\{Editing Dimension\}} type and state the basis for your determination; \textbf{(3)} Based on the given video, specify the \textit{\{Editing Dimension\}} and provide the criteria for this decision; \textbf{(4)} Identify the \textit{\{Editing Dimension\}} of the given video and explain the basis for your choice.\\
        \midrule
        \midrule
        \multicolumn{2}{c}{\textit{Editing Dimension = Shot Type, Cut Type}}\\
        \midrule
        \midrule
        Judging
        & \textbf{(1)} Based on the given video, what is the \textit{\{Editing Dimension\}} used in the given video, and what is its function? \textbf{(2)} Based on the given video, what kind of \textit{\{Editing Dimension\}} do you observe in the given video, and what function does it serve; \textbf{(3)} Determine the type of \textit{\{Editing Dimension\}} shown in the given video and elaborate on its purpose in enhancing the video's flow; \textbf{(4)} Based on the given video, Decide the \textit{\{Editing Dimension\}} used in the vide, and what role does it play in the given video?\\
        \bottomrule
    \end{tabular}
    \label{tab:question_list}
\end{table*}
\noindent
\textbf{Knowledge Base Construction}: Details about key attributions and functions can refer to the knowledge base JSON files we attached in the supplementary material. For the knowledge construction process, except for transition which has more than 70 types of transition and has no detailed and formal definition of each type, we collect definitions and functions of each component from the lecture notebook and polish the definition into detailed, non-overlapped definitions and functions. For the transition effect knowledge base, we sampled one video from each transition type and asked Gemini to give an abstract definition of the transition type based on the prompt in Figure~\ref{fig:ann_prompt}.

\noindent
\textbf{Automatic annotation} Each video in the reasoning and judging tasks are rewritten into a video-specific answer based on the prompt provided in Section~\ref{sec: supp_prompt}.

\section{Prompt}
\label{sec: supp_prompt}
\begin{figure*}
    \centering
    \includegraphics[width=0.8\linewidth]{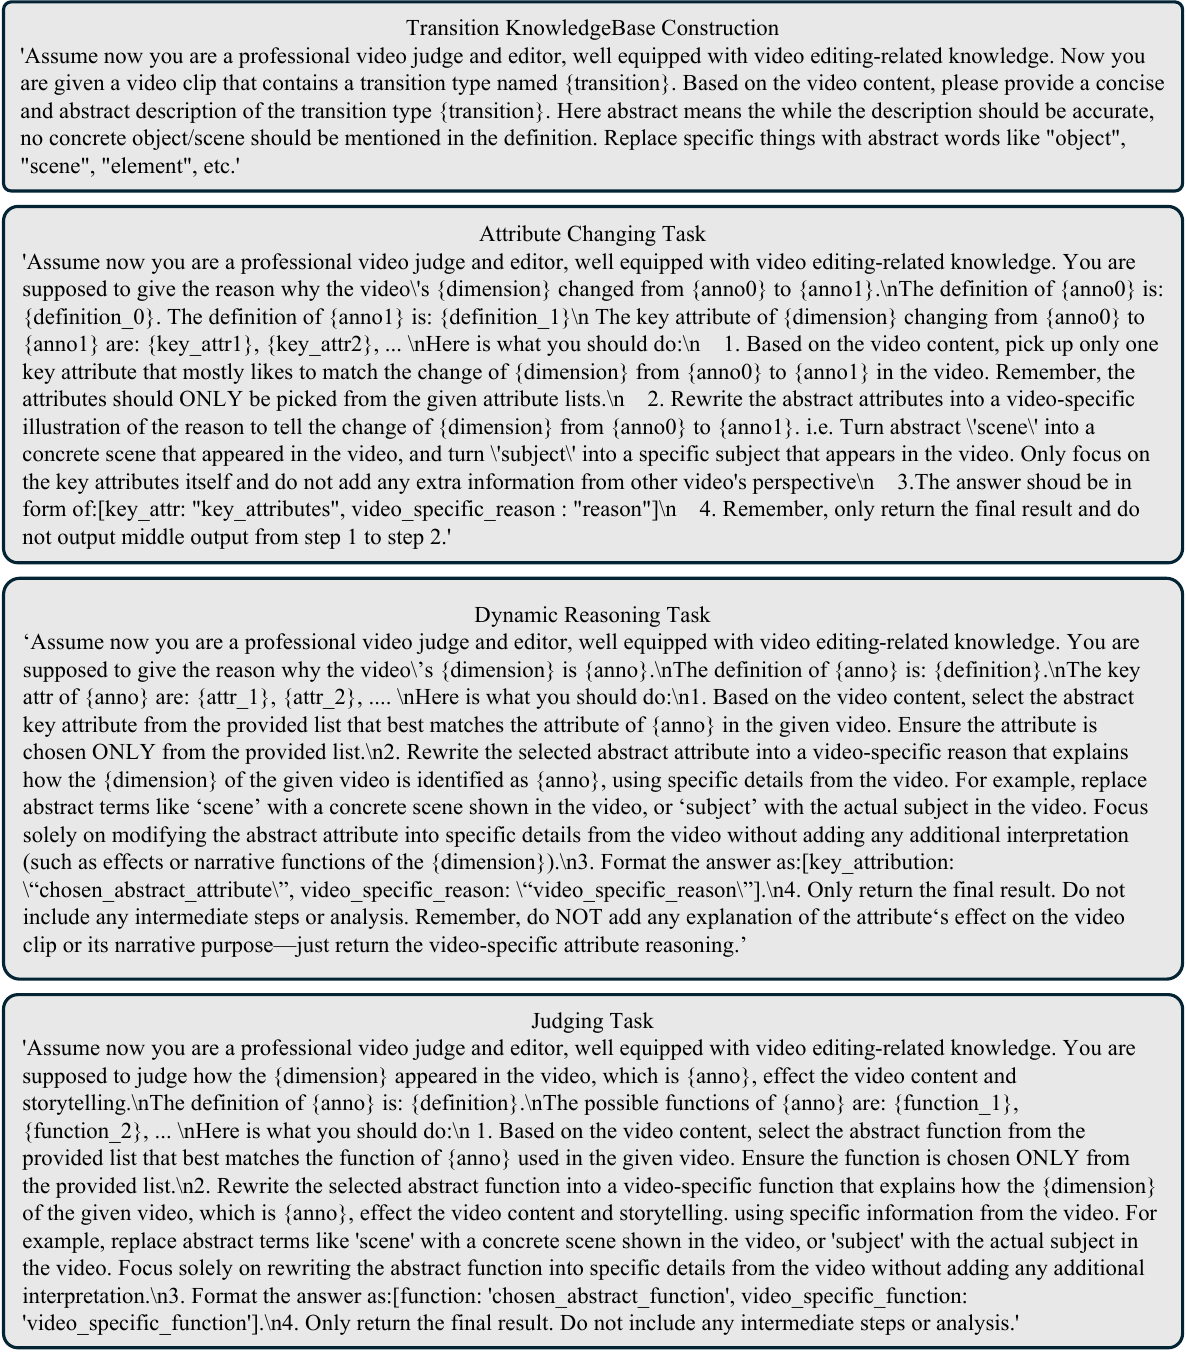}
    \caption{Annotation prompt we used in the dataset generation stage.}
    \label{fig:ann_prompt}
\end{figure*}

\begin{figure*}
    \centering
    \includegraphics[width=0.8\linewidth,height=22cm]{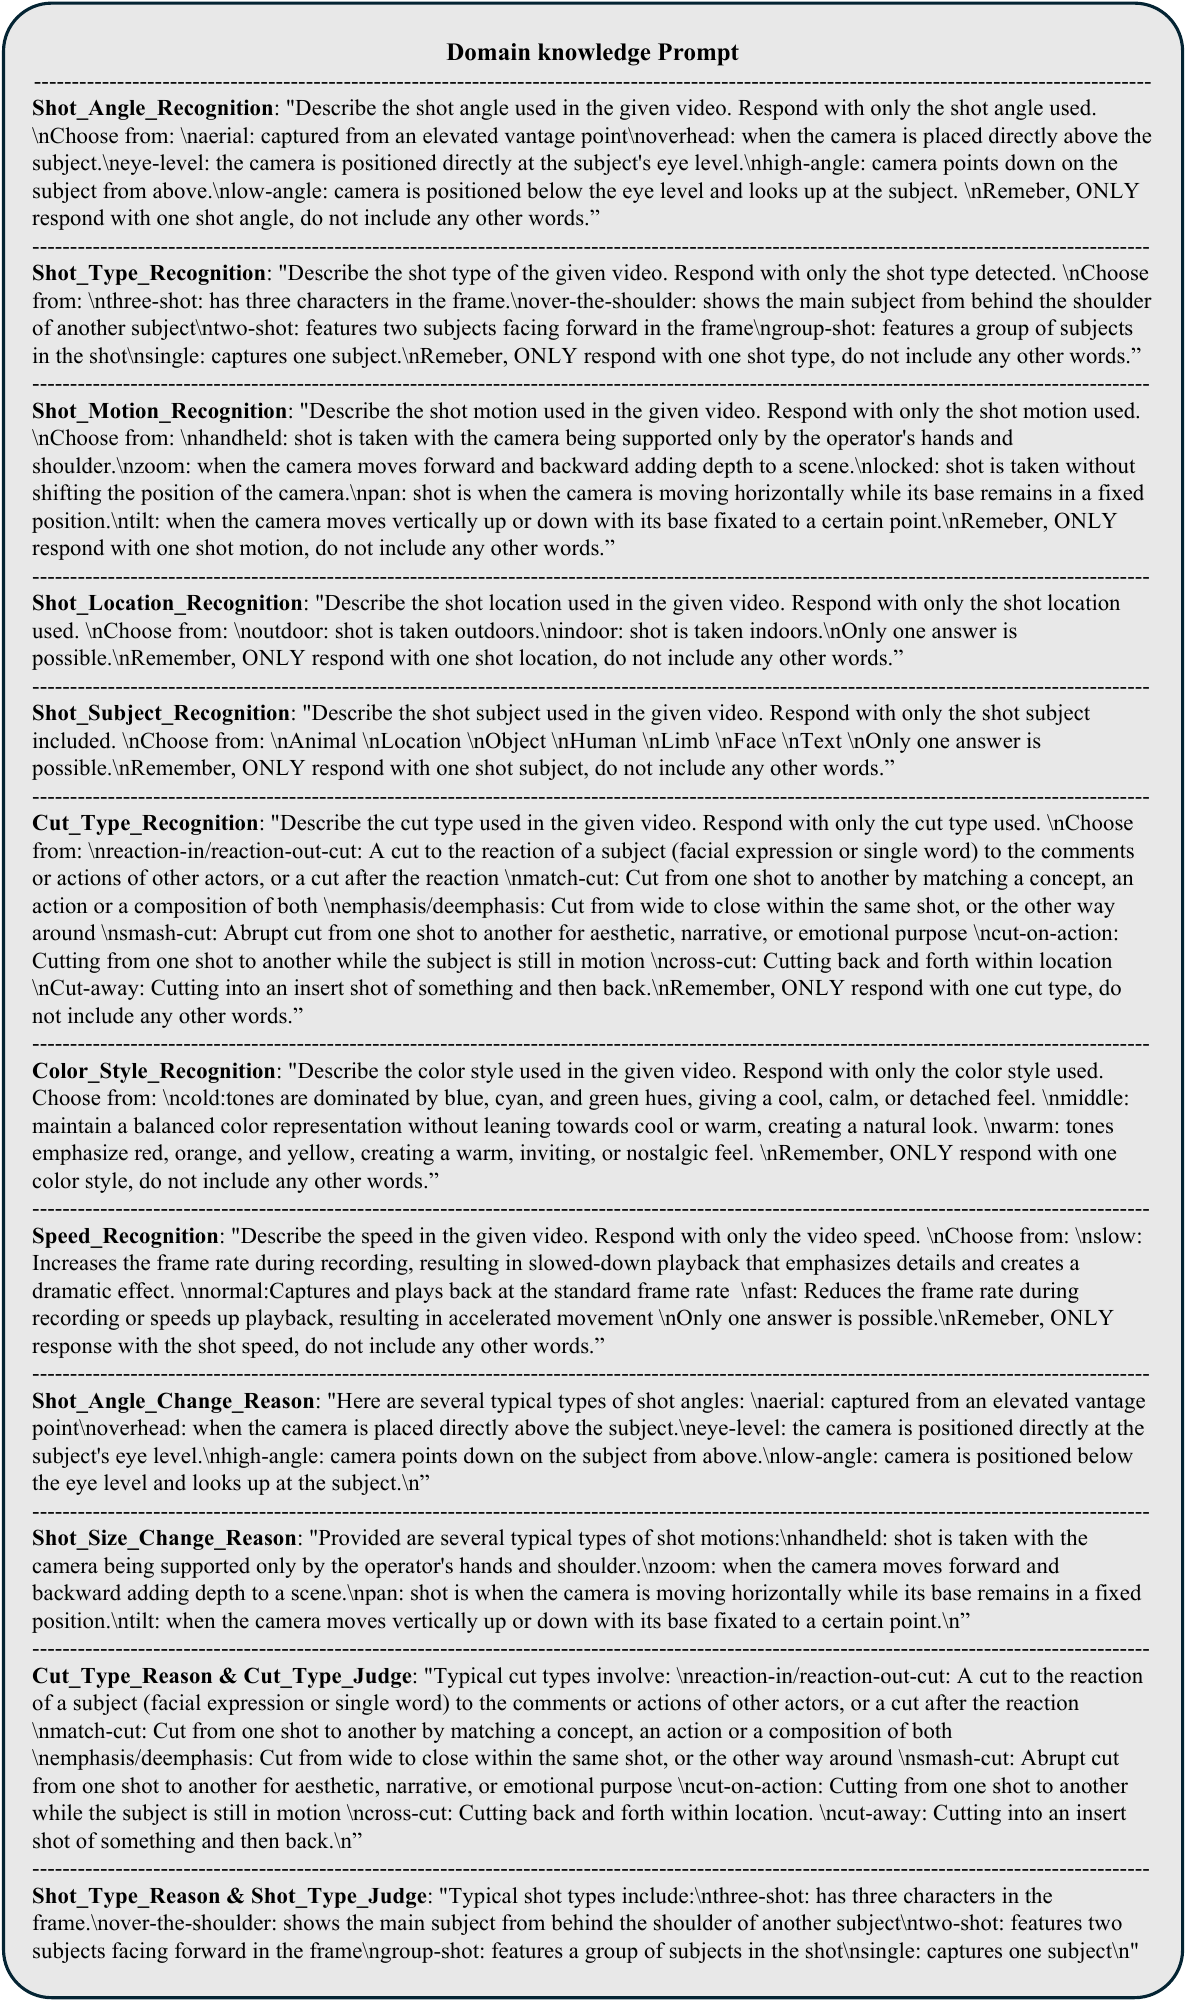}
    \caption{Task prompt we used in the inference stage.}
    \label{fig:task_prompt}
\end{figure*}

\begin{figure*}
    \centering
    \includegraphics[width=0.8\linewidth]{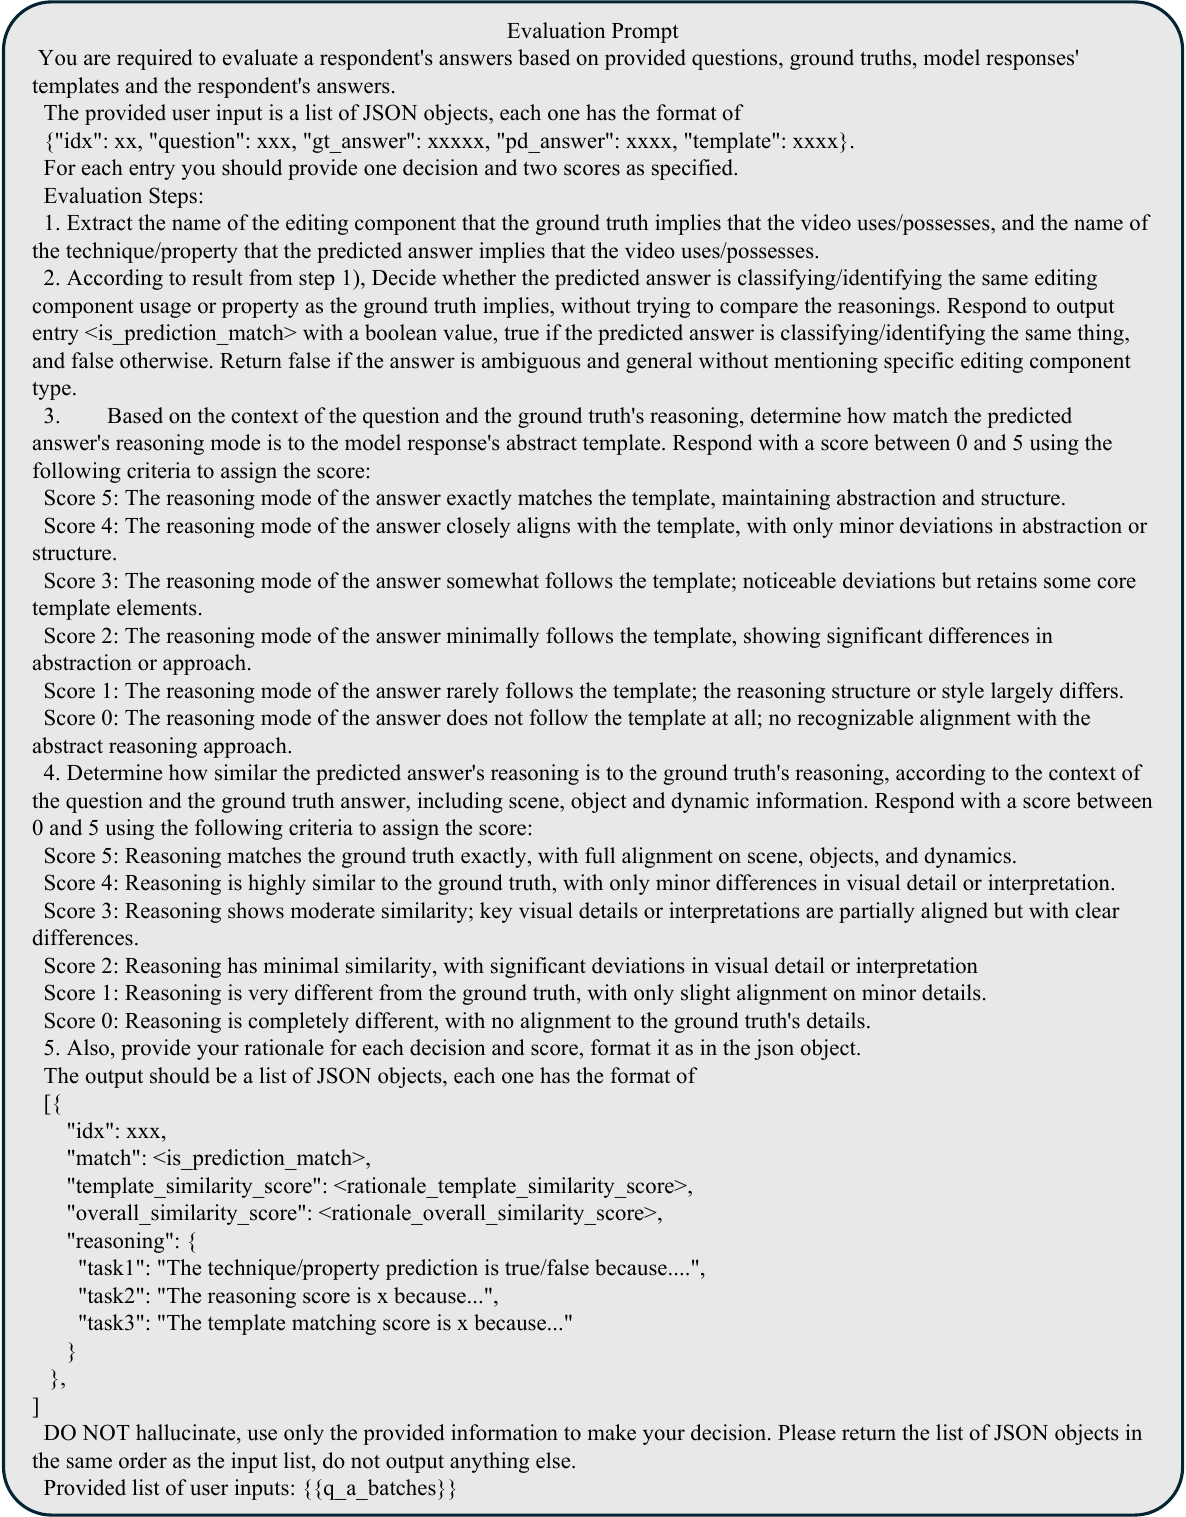}
    \caption{Evaluation prompt we used in the dataset evaluation stage.}
    \label{fig:eval_prompt}
\end{figure*}
In this section, we present the prompts covering three aspects: annotation prompt in Figure~\ref{fig:ann_prompt}, task inference prompt in Figure~\ref{fig:task_prompt}, and result evaluation prompt in Figure~\ref{fig:eval_prompt}.

\section{VEU Data as instruction tuning data}
\label{sec: supp_train_data}
\begin{table}[h!]
\centering
\caption{The impact of different task type proportions in training data on model performance. Due to complexity and diversity, data of \textbf{reasoning tasks} lead to best performance.}
\resizebox{\columnwidth}{!}{
\begin{tabular}{ccc|ccccc}
\toprule
Rec(\%) & Rea(\%) & Jud(\%) & Rec & Reason & Jud & Overall \\
\midrule
0 & 0 & 0 & 2.33 & 1.24 & 1.54 & \textbf{1.82} \\
\midrule
100 & 0 & 0 & 3.15 & 1.51 & 2.51 & \textbf{2.44} \\
0 & 100 & 0 & 2.70 & 2.24 & 2.75 & \textbf{2.53} \\
0 & 0 & 100 & 2.55 & 1.74 & 2.99 & \textbf{2.28} \\
\midrule
50 & 50 & 0 & 3.05 & 1.92 & 1.91 & \textbf{2.48} \\
0 & 50 & 50 & 2.60 & 1.90 & 2.50 & \textbf{2.32} \\
50 & 0 & 50 & 3.00 & 1.51 & 2.34 & \textbf{2.35} \\
\midrule
33 & 33 & 33 & 2.95 & 1.83 & 2.47 & \textbf{2.46} \\
\bottomrule
\end{tabular}
}
\label{tab:data_portion}
\end{table}
We investigate the effect of data from different-level tasks serving as instruction tuning data on VEU-Bench. As shown in Table~\ref{tab:data_portion}. We have the following observations. \textbf{(1)} The coverage of dimensions in the training data is crucial. While judging data involves more complex reasoning tasks, its dimensional limitations result in a 7\% gap in overall performance compared to recognition data, which covers all dimensions. \textbf{(2)} Reasoning data encompasses more comprehensive dimensions and serves as an upgrade of recognition tasks. Therefore, under the same amount of single-task training data, reasoning data achieves the best performance on VEU-Bench, 4.5\% higher than recognition data and 11.0\% higher than judging data. \textbf{(3)} By leveraging simple recognition tasks, the model gains great improvement compared to base model Qwen2-VL\cite{wang2024qwen2}. \textbf{(4)} Regarding task dimensions, the data for each task type has the strongest impact on improving performance within its respective task while reasoning data shows the best effect in enhancing performance across other tasks.

In future work, we will further expand judging-type data to achieve training datasets that balance both diversity and complexity.

\section{Details of Concept Experiment}
\label{sec: supp_concept_exp}
\begin{table*}[ht]
    \centering
    \small
    \caption{QA samples of \textbf{Concept Experimen}t across 10 dimensions}
    \begin{tabular}{l|p{5cm}|p{8cm}}
        \toprule
        Dimension & Question & Answer \\ 
        \midrule
        Shot Angle 
        & Can you describe the characteristics of a high-angle shot and how it might influence the viewer's perception of the subject? 
        & A high-angle shot is when the camera points down on the subject from above, making the subject appear smaller and potentially conveying vulnerability. \\
        \midrule
        Shot location
        & Can you describe the characteristics of an exterior shot and how it might influence the viewers perception of the setting?
        & An exterior shot is taken outdoors and typically helps establish the setting or introduce environmental elements crucial to the scene. \\
        \midrule
        Shot Motion
        & What is a tilt shot, and when would a video editor choose to use this in a scene?
        & A tilt shot involves moving the camera vertically up or down, often used to emphasize height or follow vertical motion within a scene. \\
        \midrule
        Shot Size
        & Explain what a medium shot is and how it affects the balance between subject and environment.
        & A medium shot frames the subject approximately from the waist up, allowing a balance between the subject's facial expressions and the surrounding environment. \\
        \midrule
        Shot Size
        & Explain what a medium shot is and how it affects the balance between subject and environment.
        & A medium shot frames the subject approximately from the waist up, allowing a balance between the subject's facial expressions and the surrounding environment. \\
        \midrule
        Shot Color
        & What does shot color mean in the context of video editing?
        & shot color refers to the overall color tone or palette used in a specific shot, which can convey mood, emotion, and narrative context. \\
        \midrule
        Shot Speed
        & What does slow motion mean in the context of video editing?
        & Filming at a higher frame rate to achieve slow motion when played back at a normal rate. \\
        \midrule
        Shot Type
        & Describe the use of group shots in video editing. What effect do they have on the viewer's perception of character dynamics?
        & A group shot features multiple subjects within the frame, emphasizing the relationships or dynamics between characters. \\
        \midrule
        Cut
        & What is an Emphasis Cut in the context of video editing?
        & Cut from wide to close within the same shot or the other way around. \\
        \midrule
        Transition
        & What is a Transition in the context of video editing?
        & Move from one shot to the next with special visual effects, creating a smooth or intentional visual effect as one clip changes to another. \\
        \bottomrule
    \end{tabular}
    \label{tab:concept_sample}
\end{table*}
In Table~\ref{tab:concept_sample}, we provide the 10 question samples from the concept experiment, covering all dimensions within video editing understanding and listing answers from the best model and worst model on the benchmark. It is evident that all these models have shown good responses and got high scores from human judgment as shown in Table~\ref{tab:concept_experiment}. Volunteers evaluate the answer based on the following criteria: \textit{``Given the definition of an editing element and the model’s response regarding that element, evaluate whether the model has accurate knowledge of the specified editing element and assign a score based on the degree of alignment. \textbf{Good (3):} The model provides a comprehensive definition that aligns closely with the given answer. \textbf{Middle (2):} The model’s response partially aligns with the definition but lacks specific details. \textbf{Bad (1):} The model’s response does not align at all, indicating a lack of understanding of the concept."}

\section{More Result}
\subsection{Category-wise analysis}
\label{sec: supp_analysis}
We list category-wise comparison of recognition tasks among Oscars, Qwen2-VL and Gemini Figure~\ref{fig:multi_tables}. Training on the Oscar dataset enables the model to gain a more balanced and comprehensive understanding of various categories within each editing dimension. Cases where certain elements in dimensions such as Shot Motion, Shot Angle, and Shot Type have zero recognition accuracy, as observed in Qwen2-VL, are significantly reduced. Compared to Gemini, Oscar also demonstrates more robust comprehension capabilities. For intra-shot and intra-frame element understanding, Oscars excels at distinguishing fine-grained categories, such as Extreme-close-up and Close-up in Shot Size, and Overhead and High-angle in Shot Angle. When recognizing categories that involve both video semantics and visual information synthesis, such as Cross-cut and Emphasis Cut, Oscars shows an improvement of over 30\% on average compared to the baseline model Qwen2-VL and performs comparably to the commercial model Gemini. Since the Transition task includes more than 70 categories, it is not included here. Randomly sampled multiple-choice questions effectively reflect the model’s performance in understanding transition types.
\begin{figure*}[htbp]
    \centering
    \begin{minipage}{\linewidth}
        \centering
        \begin{tabular}{cccc}
        \vspace{15pt}
        
            % First Row of Tables
            \begin{minipage}[t]{0.45\linewidth}
                \centering
                \begin{tabular}{l|cccccc}
                    \toprule
                    \multirow{2}{*}{\textbf{Model}} & \multicolumn{5}{c}{\textbf{Shot Size Recognition}} \\
                    \cmidrule{2-6}
                    ~              & \textbf{EW} & \textbf{W} & \textbf{ECU} & \textbf{M} & \textbf{CU} \\
                    \midrule
                    Qwen2-VL       & 1                  & 82         & 32                      & 37            & 89             \\
                    Gemini-Pro     & 26                  & 28         & 87                      & 82            & 58             \\
                    \rowcolor{Gray!30} Oscars         & 92                  & 22         & 94                      & 72            & 61     \\
                    \bottomrule
                \end{tabular}
            \end{minipage} &
            \hspace{5pt}
            \begin{minipage}[t]{0.45\linewidth}
                \centering
                \begin{tabular}{l|ccccc}
                    \toprule
                    \multirow{2}{*}{\textbf{Model}} & \multicolumn{5}{c}{\textbf{Shot Angle Recognition}} \\
                    \cmidrule{2-6}
                    ~ & \textbf{O} & \textbf{H} & \textbf{L} & \textbf{E} & \textbf{A} \\
                    \midrule
                    Qwen2-VL   & 63 & 0 & 29 & 82 & 79 \\
                    Gemini-Pro & 43 & 61 & 59 & 67 & 0 \\
                    \rowcolor{Gray!30}Oscars     & 76 & 20 & 35 & 63 & 68 \\
                    \bottomrule
                \end{tabular}
            \end{minipage} \\ 
            % Add vertical space between rows
        \end{tabular}
        \vspace{15pt}
        \begin{tabular}{cccc}
            % Second Row of Tables
            \begin{minipage}[t]{0.45\linewidth}
                \centering
                \begin{tabular}{l|ccccc}
                    \toprule
                    \multirow{2}{*}{\textbf{Model}} & \multicolumn{5}{c}{\textbf{Shot Type Recognition}} \\
                    \cmidrule{2-6}
                    ~ & \textbf{Th} & \textbf{Tw} & \textbf{S} & \textbf{OTS} & \textbf{G} \\
                    \midrule
                    Qwen2-VL   & 75 & 79 & 76 & 0 & 72 \\
                    Gemini-Pro & 79 & 77 & 92 & 36 & 91 \\
                    \rowcolor{Gray!30}Oscars     & 85 & 76 & 86 & 47 & 71 \\
                    \bottomrule
                \end{tabular}
            \end{minipage} &
            \hspace{5pt}
            \begin{minipage}[t]{0.45\linewidth}
                \centering
                \begin{tabular}{l|ccccc}
                    \toprule
                    \multirow{2}{*}{\textbf{Model}} & \multicolumn{5}{c}{\textbf{Shot Motion Recognition}} \\
                    \cmidrule{2-6}
                    ~ & \textbf{H} & \textbf{Z} & \textbf{L} & \textbf{T} & \textbf{P} \\
                    \midrule
                    Qwen2-VL   & 1 & 1 & 74 & 4 & 61 \\
                    Gemini-Pro & 25 & 32 & 74 & 19 & 29 \\
                    \rowcolor{Gray!30}Oscars     & 13 & 13 & 67 & 28 & 54 \\
                    \bottomrule
                \end{tabular}
            \end{minipage}
        \end{tabular}
        \vspace{15pt}
        \begin{tabular}{cccc}
            % Second Row of Tables
            \begin{minipage}[t]{\linewidth}
                \centering
                \begin{tabular}{l|ccccccccc}
                    \toprule
                    \multirow{2}{*}{\textbf{Model}} & \multicolumn{8}{c}{\textbf{Shot Subject Recognition}} \\
                    \cmidrule{2-9}
                    ~ & \textbf{Object} & \textbf{Animal} & \textbf{Cartoon} & \textbf{Location} & \textbf{Limb} & \textbf{Human} & \textbf{Face} & \textbf{Text} \\
                    \midrule
                    Qwen2-VL   & 5  & 45 & 0    & 85 & 56 & 7  & 94 & 100 \\
                    Gemini-Pro & 66 & 59 & 0    & 77 & 58 & 85 & 98 & 100 \\
                    \rowcolor{Gray!30}Oscars     & 73 & 5  & 9 & 87 & 68 & 85 & 97 & 100 \\
                                        \bottomrule
                \end{tabular}
            \end{minipage} \\ 
        \end{tabular}
        \vspace{15pt}
        \begin{tabular}{cccc}
            % Second Row of Tables
            \begin{minipage}[t]{0.45\linewidth}
                \centering
                \begin{tabular}{l|cc}
                    \toprule
                    \multirow{2}{*}{\textbf{Model}} & \multicolumn{2}{c}{\textbf{Shot Location Recognition}} \\
                    \cmidrule{2-3}
                    ~ & \textbf{Indoor Shot} & \textbf{Outdoor Shot}\\
                    \midrule
                    Qwen2-VL   & 75 & 79 \\
                    Gemini-Pro & 79 & 77 \\
                    \rowcolor{Gray!30}Oscars & 85 & 76 \\
                    \bottomrule
                \end{tabular}
            \end{minipage} &
            \hspace{5pt}
            \begin{minipage}[t]{0.45\linewidth}
                \centering
                \begin{tabular}{l|ccccc}
                    \toprule
                    \multirow{2}{*}{\textbf{Model}} & \multicolumn{5}{c}{\textbf{Shot Motion Recognition}} \\
                    \cmidrule{2-6}
                    ~ & \textbf{H} & \textbf{Z} & \textbf{L} & \textbf{T} & \textbf{P} \\
                    \midrule
                    Qwen2-VL   & 1 & 1 & 74 & 4 & 61 \\
                    Gemini-Pro & 25 & 32 & 74 & 19 & 29 \\
                    \rowcolor{Gray!30}Oscars     & 13 & 13 & 67 & 28 & 54 \\
                    \bottomrule
                \end{tabular}
            \end{minipage} \\ 
        \end{tabular}
        \begin{tabular}{cccc}
            % Second Row of Tables
            \begin{minipage}[t]{\linewidth}
                \centering
                \begin{tabular}{l|cccccccc}
                    \toprule
                    \multirow{2}{*}{\textbf{Model}} & \multicolumn{7}{c}{\textbf{Cut Type Recognition}} \\
                    \cmidrule{2-8}
                    ~ & \textbf{match-cut} & \textbf{cross-cut} & \textbf{reaction cut} & \textbf{smash-cut} & \textbf{emphasis cut} & \textbf{cut-on-action} & \textbf{cut-away} \\
                    \midrule
                    Qwen2-VL   & 7 & 3 & 100 & 3 & 3 & 0 & 0 \\
                    Gemini-Pro & 7 & 3 & 3 & 67 & 33 & 57 & 53 \\
                    \rowcolor{Gray!30}Oscars     & 1 & 21 & 73 & 3 & 67 & 7 & 30 \\
                    \bottomrule
                \end{tabular}
            \end{minipage} \\ 
        \end{tabular}
    \end{minipage}
    \caption{Category-wise Performance comparison among Oscars, Qwen2-VL~\cite{wang2024qwen2} and Gemini~\cite{team2023gemini}.}
    \label{fig:multi_tables}
\end{figure*}

\subsection{Details of Performance on general Benchmarks}
 We present the full set results on Tempcompass and Video-MME(short) in \cref{table:tempcompass} and \cref{table:videomme}. Fine-tuning on VEU data alone enables our model to outperform base model, achieving overall 6.7\% improvement on TempCompass benchmark and 2.4\% improvement on Video-MME benchmark.
\begin{table}[h]
    \centering
    \caption{Full performance comparison on TempCompass.}
    \resizebox{\linewidth}{!}{
    \begin{tabular}{l|cccccc}
        \toprule
        Model & action & direction & speed & order & attribute change & Avg.\\
        \midrule
        Qwen2-VL & 74.6 & 39.7 & 43.4 & 54.1 & 53.7 & 53.2 \\
        \rowcolor{gray!30} Oscars   & 80.8 & 46.7 & 47.6 & 62.6 & 61.4 & 59.9 \\
        \bottomrule
    \end{tabular}}
    \label{table:tempcompass}
\end{table}

\begin{table}[h]
    \centering
    \caption{Full performance comparison on on VideoMME.}
    \resizebox{\linewidth}{!}{
    \begin{tabular}{l|cccccccccccc|c}
        \toprule
        Model & CP & IS & ARec & ORec & ORea & AP & TR & ARea & OCR & SP & TP & SR & Avg.\\
        \midrule
        Qwen2-VL & 40.0 & 82.9 & 72.3 & 63.1 & 72.5 & 73.0 & 61.5 & 68.7 & 78.9 & 76.7 & 83.3 & 81.5 & 67.6\\
        \rowcolor{gray!30} Oscars   & 43.2 & 86.6 & 76.6 & 67.9 & 68.8 & 80.3 & 69.2 & 65.6 & 89.5 & 66.7 & 77.8 & 81.5 & 70.0\\
        \bottomrule
    \end{tabular}}
    \label{table:videomme}
\end{table}

\subsection{Evaluation Time Estimation}
For benchmark evaluation time estimation, we present the answer generation time cost in \cref{table:time}, while the answer scoring process is conducted by a single model, taking an average of 25 minutes to complete. Notably, the answer generation time varies depending on model size and efficiency. On average, the evaluation can be completed within 1 hour.
\begin{table}[htp]
    \centering
    \vspace{-1.0em}
    \caption{Time for Evaluation on a single A100-SXM GPU (min).}
    \vspace{-0.8em}
    \scalebox{0.8}{ % Scale the entire table to 60%
    \begin{tabular}{cccc}
        \toprule
        Qwen2-VL & MiniCPM-V & GPT4o & Gemini-1.5-pro \\
        \midrule
        45 & 32 & 40 & 33 \\
        \bottomrule
    \end{tabular}}
    \label{table:time}
\end{table}

\section{Qualitative sample of each dimension data}
\label{sec: supp_qualitative samples}
\begin{figure*}[ht]
    \centering
    \includegraphics[width=\textwidth]{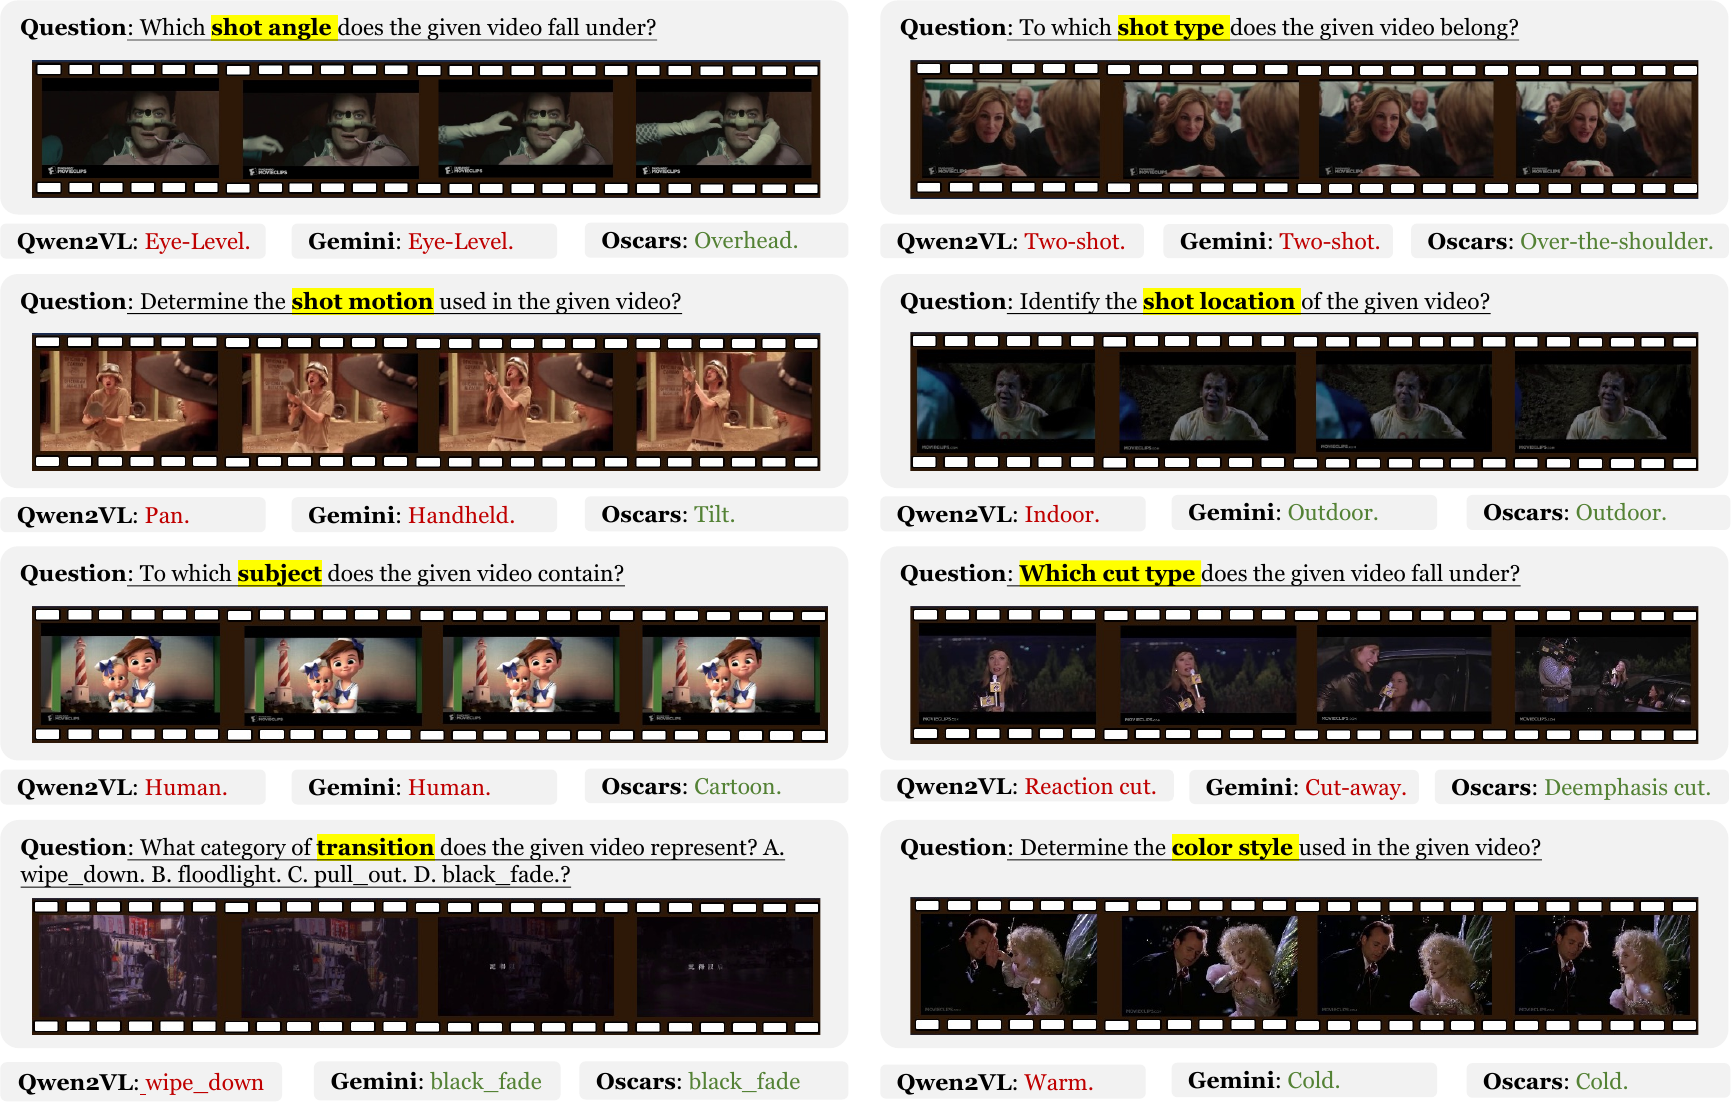}
    \caption{Qualitative result of Oscars on \textbf{recognition task} compared to Qwen2-VL~\cite{wang2024qwen2} and Gemini~\cite{team2023gemini}}
    \label{fig:rec_sample}
\end{figure*}
\begin{figure*}[ht]
    \centering
    \includegraphics[width=0.8\linewidth,height=22cm]{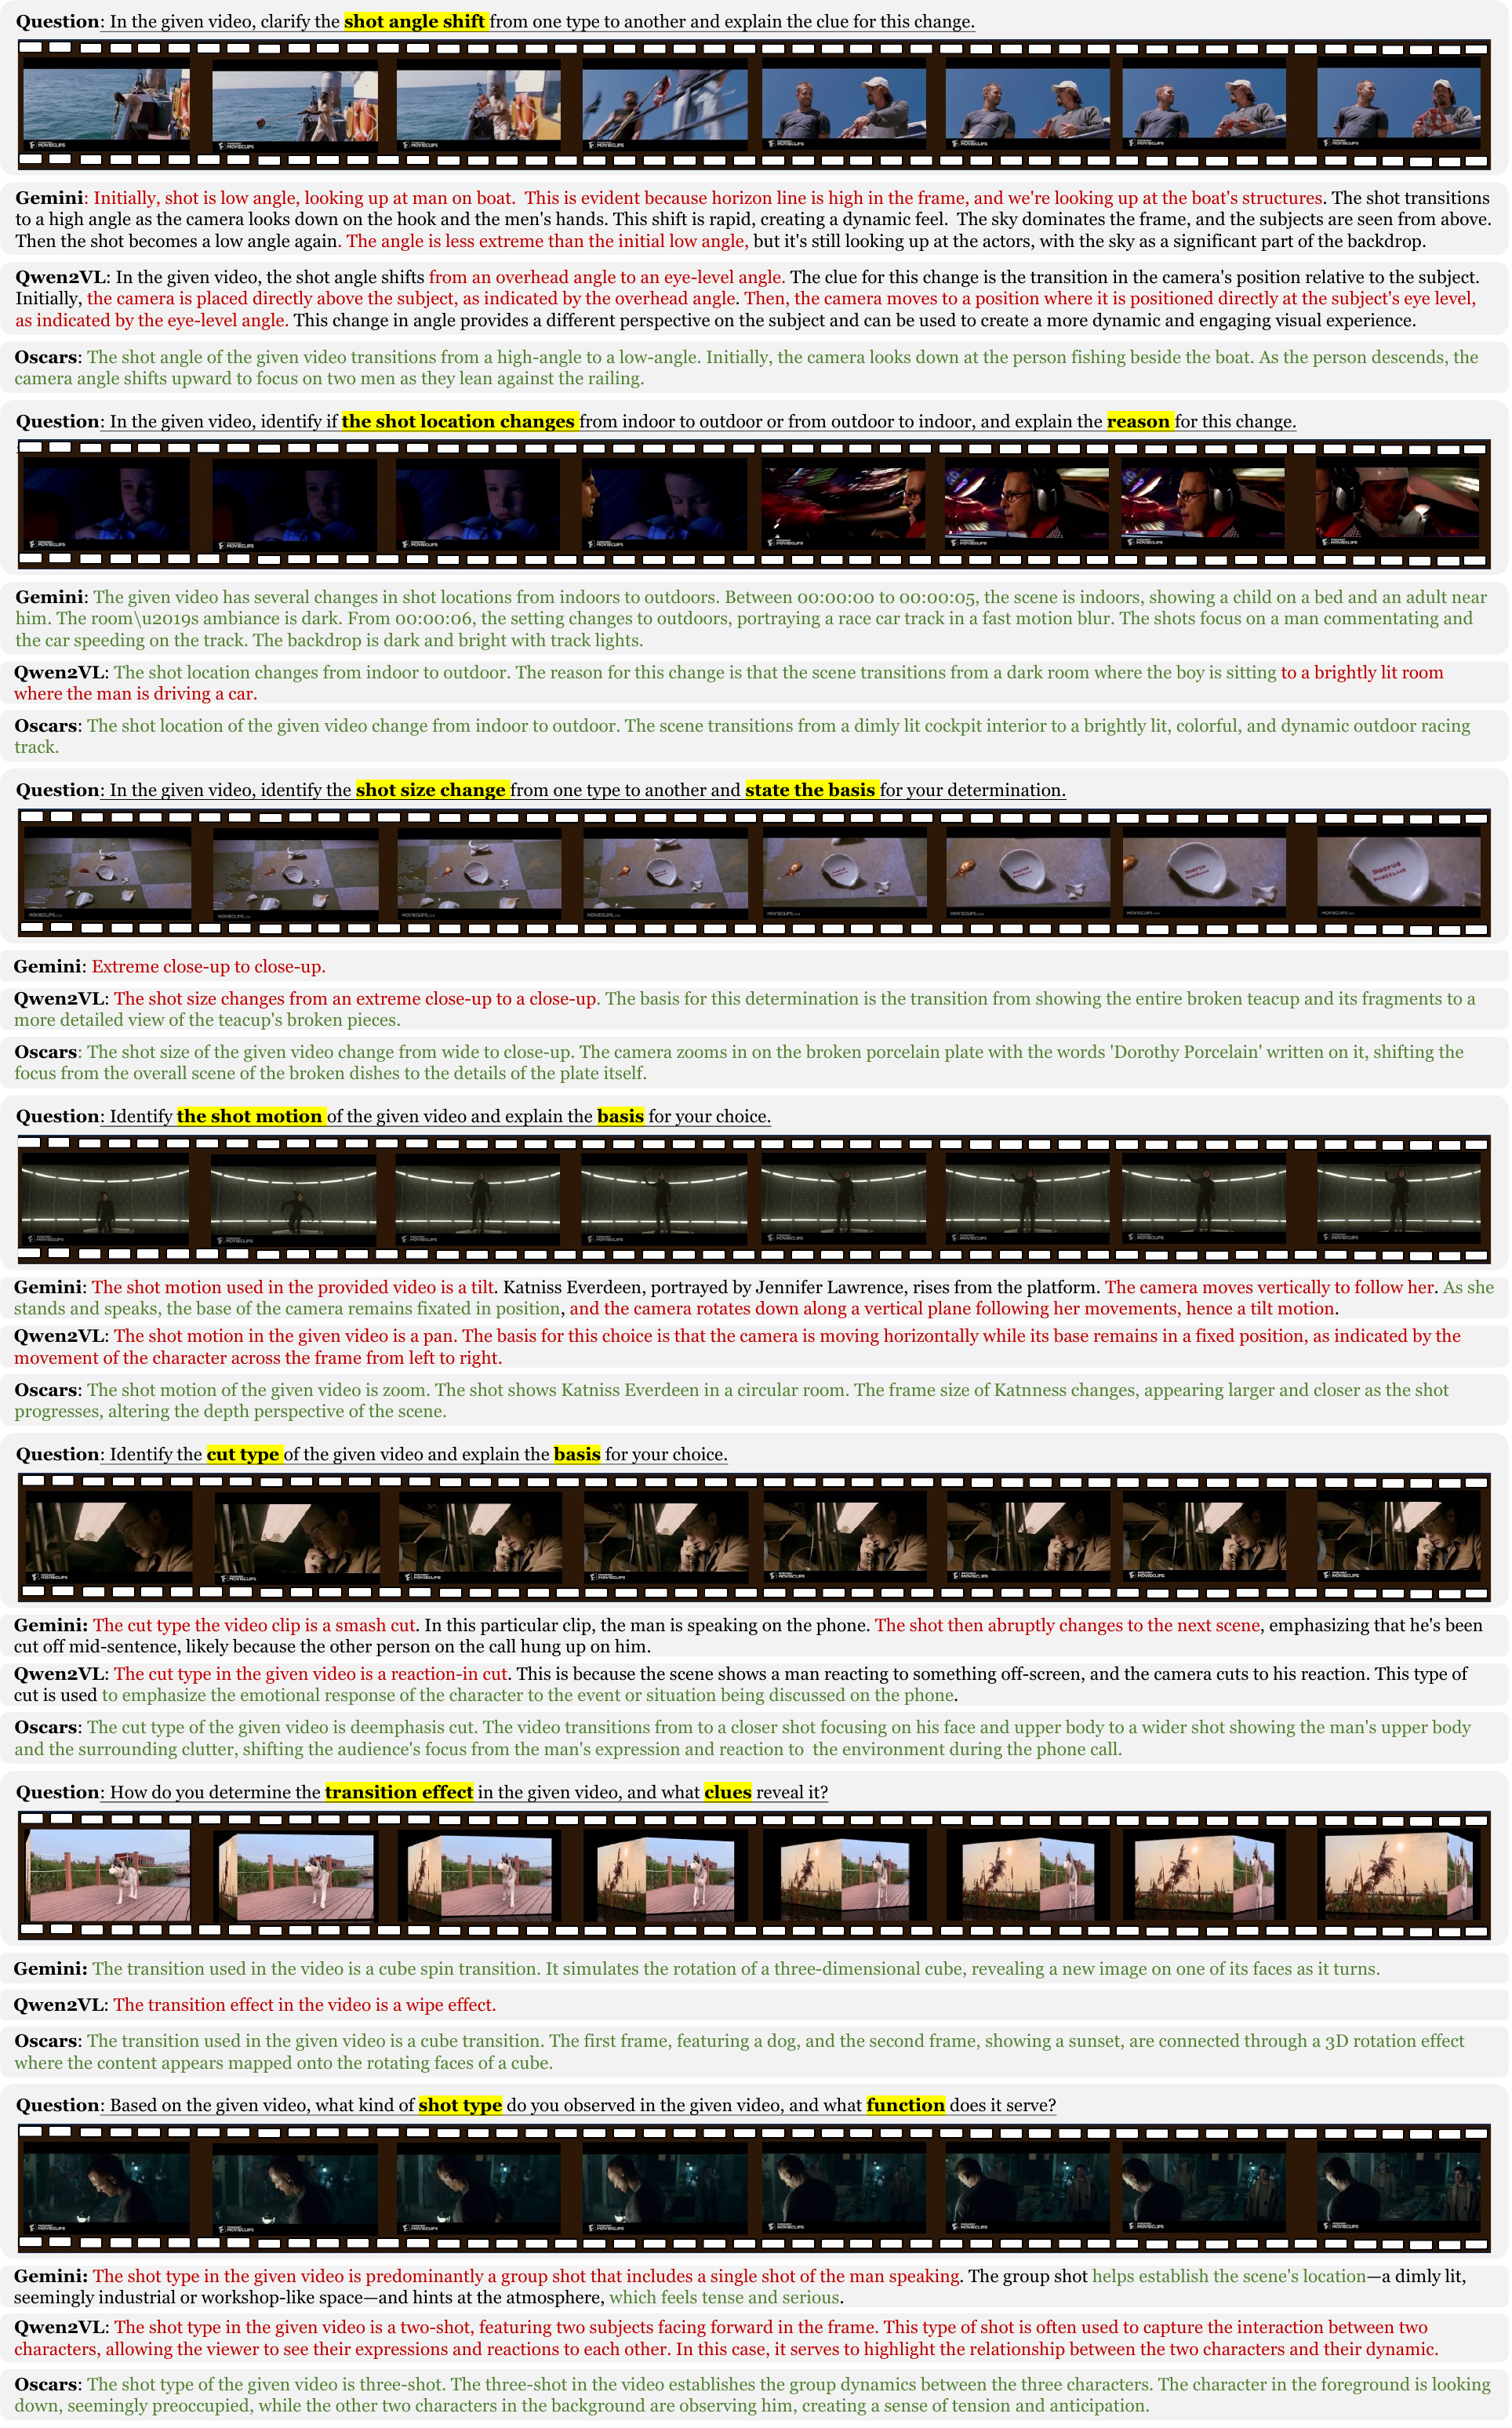}
    \caption{Qualitative result of Oscars on \textbf{reasoning and Judging tasks} compared to Qwen2-VL~\cite{wang2024qwen2} and Gemini~\cite{team2023gemini}}
    \label{fig:rea_sample}
\end{figure*}

Additional qualitative results are presented in Figure~\ref{fig:rec_sample} and Figure~\ref{fig:rea_sample}. Compared with Qwen2-VL~\cite{wang2024qwen2} and Gemini~\cite{team2023gemini}, Oscars performs admirably across a range of tasks in VEU-Bench. Oscars demonstrate the ability to capture nuanced differences between editing components and reason through video context, showcasing excellent video editing understanding and abstract visual reasoning capabilities.

\section{Limitations and Future Work}
\label{sec: supp_limitation}
Due to the limitations of current mainstream video models in supporting audio understanding, our work focuses solely on video editing comprehension related to visual information, excluding the evaluation of audio-based editing techniques. However, audio plays a critical role in video by contributing to rhythm, narrative, and information delivery. In future research, we plan to expand the benchmark to include audio, enabling a more comprehensive evaluation of video editing understanding and holistic video comprehension capabilities.

Additionally, as noted in the section on constructing change tasks, current Vid-LLMs struggle to effectively process multiple video inputs. As a result, tasks involving the comprehension and organization of multiple video materials, which are common in editing scenarios, are not included in the current VEU-Bench evaluation. In future iterations, we aim to introduce multi-video editing understanding tasks and anticipate advancements in open-source Vid-LLMs that can better process multiple video inputs and temporal information.
